# Supplementary material for: PADME: A Deep Learning-based Framework for Drug-Target Interaction Prediction
Source: arXiv:1807.09741 ancillary file (2019-08-21)
Supplement: Supplementary file 1 [file supplementary_text.pdf]

# Supporting Information

## of

### **PADME: A Deep Learning-based Framework for Drug-Target Interaction Prediction**

Authors: Qingyuan Feng (1), Evgenia Dueva (2), Artem Cherkasov (2, 3, 4\*), Martin Ester (1,5\*)

1: School of Computing Science, Simon Fraser University, Burnaby, BC V5A1S6, Canada

2: Vancouver Prostate Centre, Vancouver, BC V6H3Z6, Canada

3: Department of Urologic Sciences, University of British Columbia, BC V5Z1M9, Canada

4\*: [artc@interchange.ubc.ca](mailto:artc@interchange.ubc.ca)

5\*: [ester@cs.sfu.ca](mailto:ester@cs.sfu.ca)

## Table of Contents

|                                                   |    |
|---------------------------------------------------|----|
| 1. Datasets preparation.....                      | 3  |
| 2. Quantitative results for oversampled data..... | 6  |
| 3. Case Studies Extended.....                     | 7  |
| 3.1. T-tests on cell lines .....                  | 10 |
| 3.2. Wet-lab experiments on compounds.....        | 13 |
| 3.3. Summary .....                                | 14 |

## 1. Datasets preparation

### **Davis dataset**

Compound names were extracted from Davis dataset [1, 2]. The corresponding compound CIDs and SMILES strings were extracted from PubChem [3]. NCBI GenBank Protein accession numbers from Davis dataset were used to download the corresponding amino acid sequences via NCBI Batch Entrez [4]. As sequences with accession numbers P0C1S8 and P0C264 were no longer available in GenBank Protein, their updated versions P0C1S8.2 and P0C264.2 were used. Protein sequences were modified according to descriptions from the original paper, e.g. mutations were introduced and only sequences corresponding to specified domains, if any, were left (domains were detected according to GenBank Protein domains annotation).

### **Metz dataset**

Kinase names extracted from Metz Dataset [5, 6] were searched in KinBase [7]. The gene names found were saved and the corresponding amino acid sequences were extracted from Human Kinome Database (downloaded from KinBase – The Kinase Database [8, 9] and containing 538 human kinases). Compounds with identical SMILES strings, but different ChEMBL IDs and activity measurement results were filtered out in the execution of the program.

### **KIBA dataset**

ChEMBL IDs and protein IDs were extracted from the KIBA dataset [10, 11]. Canonical smiles strings were loaded from ChEMBL database [12, 13] via ChEMBL web resource client [14, 15]. NCBI GenBank Protein accession numbers from KIBA dataset were used to download the corresponding sequences via NCBI Batch Entrez [4].

### **ToxCast Dataset**

The following file archives were downloaded from ToxCast website:

- 1) INVITRODB\_V2\_SUMMARY (October 2015) [16]. File Assay\_Summary\_151020.xls contains summary information about assays. File oldstyle\_ac50\_Matrix\_151020.xls contains summary of testing results.

2) DSSTox\_ToxCastRelease\_20151019 [17]. File DSSTox\_ToxCastRelease\_20151019.xls contains summary of chemicals tested.

Compound structures contained in DSSTox\_ToxCastRelease\_20151019.xls were processed using MOE 2013.8 [18] as follows: water samples, mixtures with unidentified content, and polymers were excluded; structures were “washed” with MOE: salts were split and the largest part of each salt was retained, the structures were then neutralized; compounds containing metal atoms were removed; duplicated structures were filtered using MOE sdsort tool.

Only assays with single corresponding “intended target” in the file Assay\_Summary\_151020.xls were selected and split in groups, whose Uniprot IDs were extracted and used to get protein sequences from Uniprot [19, 20].

The AR antagonist score was constructed as a linear combination of PADME predictions for assays involving AR (Table S1):

$$\begin{aligned} \text{Antagonist\_score} = & \text{NVS\_NR\_hAR} + (1/2 * \text{TOX21\_AR\_LUC\_MDAKB2\_Antagonist} + 1/2 \\ & * \text{TOX21\_AR\_BLA\_Antagonist\_ratio}) - \{ (1/2 * \text{OT\_AR\_ARSRC1\_0480} + \\ & 1/2 * \text{OT\_AR\_ARSRC1\_0960}) + \text{ATG\_AR\_TRANS\_up} + (1/3 * \text{OT\_AR\_ARELUC\_AG\_1440} + \\ & 1/3 * \text{TOX21\_AR\_LUC\_MDAKB2\_Agonist} + 1/3 * \text{TOX21\_AR\_BLA\_Agonist\_ratio}) \} \end{aligned}$$

Table S1 ToxCast assays description

| Stage                | Assay                          | Tissue / Cell lines                                     | Assay description                                                                                                                                                                                                                                                                                                                                                                                                                              |
|----------------------|--------------------------------|---------------------------------------------------------|------------------------------------------------------------------------------------------------------------------------------------------------------------------------------------------------------------------------------------------------------------------------------------------------------------------------------------------------------------------------------------------------------------------------------------------------|
| Receptor binding     | NVS_NR_hAR                     | extracted gene-proteins from LnCAP in a cell-free assay | An analysis of receptor-ligand interactions in screening applications. It utilizes a radiolabeled ligand and a source of receptor (membranes, soluble/purified). Radioligand binding competition                                                                                                                                                                                                                                               |
| Cofactor recruitment | OT_AR_ARSRC1_0480              | HEK293T, a human kidney cell line                       | Assay is used to study the interaction of two proteins. An enzyme or fluorescent protein is rationally dissected into two fragments and fused to two test proteins, whose interaction is being studied. Binding of the two test proteins results in the reconstitution of the enzyme or fluorescent protein from the two fragments.                                                                                                            |
|                      | OT_AR_ARSRC1_0960              |                                                         |                                                                                                                                                                                                                                                                                                                                                                                                                                                |
| Gene transcription   | ATG_AR_TRANS_up                | HepG2, a human liver cell line                          | mRNA Induction (also known as nucleic acid amplification method): A method that uses purified enzymes to isolate and then replicate specific nucleic acids to levels where they can be detected. Assay is designed to make measurements of mRNA induction, a form of inducible reporter, as detected with fluorescence intensity signals by Reverse transcription polymerase chain reaction (RT-PCR) and Capillary electrophoresis technology. |
| Gene expression      | OT_AR_ARELUC_AG_1440           | CHO-K1, a Chinese hamster ovary cell line               | Luciferase Induction: Luciferase gene is attached to the regulatory sequence of a gene of interest. The effect of a perturbagen on the expression of the gene of interest could be easily measured by the detection of light emitted as a product the luciferase reaction.                                                                                                                                                                     |
|                      | TOX21_AR_LUC_MDAKB2_Agonist    | MDA-kb2, a human breast cell line                       |                                                                                                                                                                                                                                                                                                                                                                                                                                                |
|                      | TOX21_AR_LUC_MDAKB2_Antagonist |                                                         |                                                                                                                                                                                                                                                                                                                                                                                                                                                |
|                      | TOX21_AR_BLA_Agonist_ratio     |                                                         |                                                                                                                                                                                                                                                                                                                                                                                                                                                |

|  |                               |                                   |                                                                                                                                                                                                                                             |
|--|-------------------------------|-----------------------------------|---------------------------------------------------------------------------------------------------------------------------------------------------------------------------------------------------------------------------------------------|
|  | TOX21_AR_BLA_Antagonist_ratio | HEK293T, a human kidney cell line | Beta lactamase gene is attached to the regulatory sequence of a gene of interest. The effect of a perturbagen on the expression of the gene of interest could be easily monitored by the detection of the product of beta lactamase enzyme. |
|--|-------------------------------|-----------------------------------|---------------------------------------------------------------------------------------------------------------------------------------------------------------------------------------------------------------------------------------------|

## 2. Quantitative results for oversampled data

As mentioned in the main text, we tried to oversample the ToxCast dataset to balance the number of active/inactive observations to boost the performance of the models. Oversampling is a technique that increases the samples of the minority class by randomly sampling the minority class samples in addition to the existing samples, such that the new dataset is more balanced, enabling the machine learning model to learn in a “healthier” way [21]. Compared to other ways to balance the dataset like undersampling, oversampling was found to be superior in convolutional neural networks [22]. Often the number of inactive samples equals the number of active ones after oversampling.

Because the 672 assays of the ToxCast dataset were divided into 61 measurements, each drug-target pair can have multiple non-null observations. Even for those drug-target pairs (only a small fraction, less than 20% of total pairs) with some active measurements, it is still very likely that most of its non-null measurements are inactive, so making half of the total measurements across all drug-target pairs active is completely distorting the dataset and infeasible. Hence, we define “active pair” as a drug-target pair that has at least one active measurement, we also define “inactive pair” as a pair that has all its non-null measurements inactive, and we randomly sampled the active pairs such that the total number of active pairs equals inactive pairs.

We used the oversampled dataset for CV. Each training fold was split from oversampled dataset without further processing, while the validation folds have their duplicate drug-target pairs removed, so that we are essentially training on oversampled data and testing on the original data. To prevent each oversampled pair from appearing in both training and validation sets, we put all repeated instances of a pair into the same fold.

Table S2 presents the 5-fold CV results of the ToxCast PADME models with oversampling, while for reference, alongside them are the CV results of ToxCast PADME models without oversampling (extracted from tables 2~3). All the hyperparameters used for training DNN on

oversampled datasets are the same as those already found for training on original datasets, so the results presented for oversampled data may not be optimal.

*Table S2 CV Results of PADME models on ToxCast original and oversampled datasets. Boldfaced numbers indicating the better results between the models trained on original VS oversampled datasets.*

|         |                                 | RMSE             |                     |                  |                     | Concordance Index |                     |                  |                     |
|---------|---------------------------------|------------------|---------------------|------------------|---------------------|-------------------|---------------------|------------------|---------------------|
|         |                                 | PADME-ECFP       |                     | PADME-GraphConv  |                     | PADME-ECFP        |                     | PADME-GraphConv  |                     |
| Dataset | Cross Validation Splitting Type | Original dataset | Oversampled dataset | Original dataset | Oversampled dataset | Original dataset  | Oversampled dataset | Original dataset | Oversampled dataset |
| ToxCast | Warm (Random)                   | <b>0.4049</b>    | 0.4887              | <b>0.4092</b>    | 0.4663              | <b>0.7908</b>     | 0.7717              | <b>0.7963</b>    | 0.7781              |
|         | Cold Drug                       | <b>0.4447</b>    | 0.5159              | <b>0.4448</b>    | 0.5057              | <b>0.7196</b>     | 0.6628              | <b>0.7329</b>    | 0.6887              |
|         | Cold Target                     | <b>0.4794</b>    | 0.5381              | <b>0.4896</b>    | 0.6554              | 0.6752            | <b>0.7008</b>       | <b>0.6979</b>    | 0.6735              |

The effect of oversampling is surprising. Clearly, oversampling overall has a negative influence on the prediction performance. We speculate that, in oversampling, the repetition of active pairs reduced the information diversity in some of the training folds, because some inactive pairs that could have been selected as training samples were “squeezed” into the validation set due to the oversampling of active pairs. A repeated (active) pair which must have all its repeated instances placed in one fold can potentially “squeeze” several unique pairs out of the fold, possibly this phenomenon cancels out the positive effects of oversampling. Because imbalanced dataset is a very common scenario and important problem in virtual screening, more studies of ToxCast regarding this issue might be needed.

### 3. Case Studies Extended

We conducted more case studies than presented in the main text. But since we are yet to satisfactorily interpret the results, they are presented here.

Those case studies were performed to further validate the predictions of PADME using the NCI60 cell line dataset and drug response. Specifically, we investigated whether the compounds predicted with strong AR antagonist effects could inhibit proliferation of related cancer cell lines.

As mentioned in the main text, we used all compounds in all the datasets studied in this paper, including those in the NCI60 dataset, and AR as the only target protein. For prediction, we took the average of the predictions of PADME-ECFP and PADME-GraphConv, from which we calculated AR antagonist scores, the formula was presented in the “Dataset Preparation” section in the Supporting Information. We expect the compounds with higher AR antagonist scores to show stronger activity in NCI60 dataset. We also calculated AR agonist scores (not presented due

to similar results obtained). Among the measurements in NCI60, we only considered the logGI50 values, which are also real numbers. The smaller the logGI50 value, the more active the compound is in suppressing the growth of cancer cells. GI stands for “Growth Inhibition”.

The formula for calculating AR antagonist score was based on assumption, which introduces another layer of complexity to the prediction. The AR binding prediction results presented in the main text demonstrated the reliability of PADME, while the unsatisfactory results presented here could be due to problems in the formula itself and the intrinsic difficulty with cell-based assays, not the problem with PADME. In fact, as we will mention later, PADME faithfully captures the pattern from the training data.

Based on previous researches showing the relationship between AR and breast cancer [23], we hypothesized that the AR antagonist (or agonist) scores should have a strong correlation with logGI50 values of the breast cancer cell lines and a lower correlation with logGI50 values of other cancer cell lines. We also assumed that the ordered list of compounds ranked by AR antagonist scores would agree well with the ordered compound list ranked by logGI50 values in breast cancer cell lines, while agreeing poorly with the compound list ranked by logGI50 values in other cancer cell lines.

To test the validity of our assumptions, we selected the compounds that appear in both ToxCast and NCI60 datasets, calculated the AR antagonist scores of those compounds using the observed values in ToxCast dataset, plotted the antagonist scores against the negative logGI50 values (taking negative to make the two values positively correlated) of the corresponding compounds in NCI60 dataset, and also measured the ranking agreement between the AR antagonist scores and logGI50 values using quantitative methods. Some results are shown in Figure S2 and Table S3.

*Figure S2 Scatter plot of AR antagonist scores VS negative logGI50 values for HS 578T cell line in breast cancer and M14 cell line in Melanoma. Each dot corresponds to a compound.*

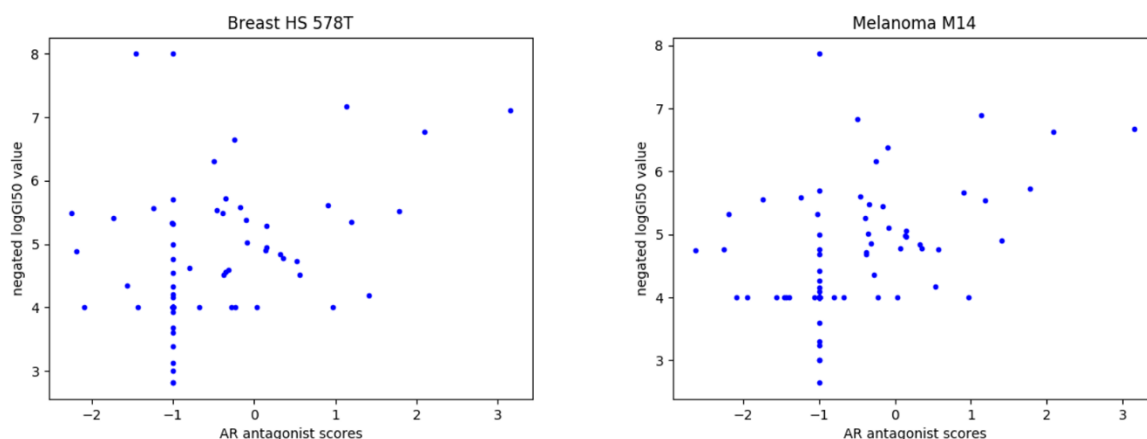

Table S3 Agreement between logGI50 values and AR antagonist scores in different cell lines.

| Panel    | Cell line       | number of valid compounds | Concordance Index | NDCG   | Spearman's correlation | p-value for Spearman's correlation |
|----------|-----------------|---------------------------|-------------------|--------|------------------------|------------------------------------|
| Prostate | PC-3            | 68                        | 0.6735            | 0.8216 | 0.5127                 | 7.82E-06                           |
| Prostate | DU-145          | 68                        | 0.6579            | 0.7915 | 0.4419                 | 1.62E-04                           |
| Colon    | HCT-116         | 85                        | 0.6757            | 0.8397 | 0.4763                 | 4.07E-06                           |
| Melanoma | M14             | 82                        | 0.6698            | 0.8554 | 0.4576                 | 1.55E-05                           |
| Breast   | MDA-MB-468      | 31                        | 0.6035            | 0.8048 | 0.2914                 | 0.1118                             |
| Breast   | HS 578T         | 68                        | 0.6081            | 0.8422 | 0.3098                 | 0.0101                             |
| Breast   | BT-549          | 61                        | 0.6768            | 0.8241 | 0.5038                 | 3.49E-05                           |
| Breast   | MCF7            | 66                        | 0.6434            | 0.8407 | 0.4050                 | 0.00074                            |
| Breast   | T-47D           | 65                        | 0.6880            | 0.7705 | 0.5388                 | 3.65E-06                           |
| Breast   | MDA-MB-231/ATCC | 65                        | 0.6601            | 0.7836 | 0.4450                 | 0.000204                           |

Because AR is strongly related to breast cancer, we assumed there should be a strong positive correlation between the AR antagonist scores and negative logGI50 values. Similarly, since Melanoma is not shown to be related to AR, we assumed there would be a much weaker (or even zero) correlation between AR antagonist scores and negative logGI50 values compared to breast cancer cell lines. However, figure S2 does not show a discernible difference between Melanoma and breast cancer. Plots of other breast cancer cell lines and other cancer types also gave us similar patterns.

In addition to visual inspection in Figure S2, we used several metrics to measure the ranking agreement between the AR antagonist scores and logGI50 values in Table S3, in which Normalized Discounted Cumulative Gain (NDCG) is a metric often used in data mining to examine the quality of ranking [24]. For NDCG we used the classical logarithmic discount, and chose zero-adjusted negative logGI50 as the relevance score of the compound, such that it starts from 0 and increases with stronger relevance. NDCG values range from 0 to 1, the higher the value is, the better the ranking quality. For Concordance Index, we used the compound list ranked by AR antagonist scores as the predicted ranking, while the compound list ranked by logGI50 value corresponds to the true ranking. Spearman's correlation is calculated on ranks only, so it is also a metric measuring the agreement between two rankings.

The colon cancer, Melanoma and the presented prostate cancer cell lines are not known to be related to AR, so they are expected to have lower agreements between logGI50 values and AR scores. However, in table S3, it can be seen that all metrics are quite similar across multiple cell lines. (More cell lines are tested on, but only a selected subset is presented in the paper. All the cell lines yielded similar results.)

We also carried out the same experiments using AR agonist score that we calculated from the observed dataset. Likewise, there are no notable differences between cell lines. The details are out of the scope of this section.

As we can see, contrary to what we expected, the compounds' antagonist effects on AR are not more strongly related to their activity in breast cancer cell lines than to their activity in other cell lines. **This phenomenon was also observed with our predicted AR antagonist scores**, which shows PADME's faithfulness, but we don't present the details here, since they are less convincing than scores calculated from true values. This suggests that either the AR is related to a wide range of cancers, or the true relationship between AR and prostate cancer is far from a linear relationship, or the assumptions used in making the AR antagonist score formula causes the problem. We suggest this as an issue for future research.

### 3.1. T-tests on cell lines

We wanted to examine our assumption that the compounds ranked high in (both predicted and observed) AR antagonist scores generally have higher activities in suppressing the growth of breast cancer cell lines. Since we already found the AR antagonist scores to have similar relationship with all cell lines, this assumption actually degenerates into a general toxicity problem. Nevertheless, we decided to take a look.

This time, we start with the predicted scores, to see whether those predicted high-ranking antagonistic compounds are truly inhibiting cancer cell lines.

We used only the Breast Cancer panel in the NCI60 dataset, in which we chose 5 out of 6 cell lines, leaving out the one with relatively few observations.

We report the results separately for each cell line. For each of them, we took the top 100, top 1000, top 15000 and all compounds according to the averaged AR antagonist score. We skipped those compounds that were absent from the cell line to ensure that the top-n set contains n compounds. Say we have a top-100 list for cell line X, the 100<sup>th</sup> compound in the list is not in the top 100 in the sorted AR antagonist score list, because there are compounds in AR score list that do not have observations for X.

We calculated the mean and standard deviation of the logGI50 values for those top-n compounds. Table S4 presents the results for some breast cancer cell lines.

*Table S4 Mean and standard deviation of logGI50 values in top-n compounds in predicted AR antagonist scores.*

| Panel  | top_n | cell line | mean value | standard deviation |
|--------|-------|-----------|------------|--------------------|
| Breast | 32128 | BT-549    | -4.6792    | 0.8742             |
| Breast | 15000 | BT-549    | -4.8765    | 0.9313             |
| Breast | 1000  | BT-549    | -5.4167    | 1.4049             |
| Breast | 100   | BT-549    | -6.7358    | 1.4517             |
| Breast | 35507 | MCF7      | -4.8237    | 1.0245             |
| Breast | 15000 | MCF7      | -5.1029    | 1.0997             |
| Breast | 1000  | MCF7      | -5.8090    | 1.5528             |
| Breast | 100   | MCF7      | -7.4770    | 1.3254             |

|        |       |                 |         |        |
|--------|-------|-----------------|---------|--------|
| Breast | 33441 | HS 578T         | -4.6970 | 0.9083 |
| Breast | 15000 | HS 578T         | -4.9178 | 0.9754 |
| Breast | 1000  | HS 578T         | -5.4224 | 1.4251 |
| Breast | 100   | HS 578T         | -6.7281 | 1.6891 |
| Breast | 33356 | T-47D           | -4.7390 | 0.9110 |
| Breast | 15000 | T-47D           | -4.9499 | 0.9534 |
| Breast | 1000  | T-47D           | -5.5650 | 1.4554 |
| Breast | 100   | T-47D           | -6.9877 | 1.4680 |
| Breast | 34819 | MDA-MB-231/ATCC | -4.6886 | 0.8960 |
| Breast | 15000 | MDA-MB-231/ATCC | -4.9206 | 0.9469 |
| Breast | 1000  | MDA-MB-231/ATCC | -5.4155 | 1.3321 |
| Breast | 100   | MDA-MB-231/ATCC | -6.5016 | 1.4729 |

Based on the values in table S4, we conducted a series of one sample t-tests. For example, in Table S5, the entry corresponding to (100, 1000) is obtained by performing a t-test on top 100 compounds against the top 1000 compounds, in which  $H_0$  is: the top 100 compounds are obtained from the top 1000 randomly. In more formal terms, the mean logGI50 values of the hypothetical group that the top 100 compounds in AR score in BT-549 dataset belong to, equals the mean of that of top 1000 compounds (-5.4167).  $H_1$  is: the top 100 compounds in AR scores are truly more active than the top 1000 compounds. In more formal terms, the mean logGI50 values of the hypothetical group that the top 100 compounds in AR score belong to, is smaller than the mean of that of top 1000 compounds (-5.4167).

We can see that the null hypotheses are all strongly rejected, which shows a consistent trend that the compounds with a high predicted AR score tend to be more actively inhibiting the prostate cancer cell lines. Similar results are also obtained on other cell lines in Table S4, but the tables are not presented here for brevity.

Table S5 Base top-k compared against other top-k's for BT-549. A one sample t-test is conducted for each filled entry, where  $H_0$  is that both top-k's have identical means, while  $H_1$  is that the base top-k has a smaller mean.

| Cell line: BT-549 | Top-k to compare against            |                                      |                                       |
|-------------------|-------------------------------------|--------------------------------------|---------------------------------------|
| Base top-k        | 1000                                | 15000                                | All (35159)                           |
| 15000             | -                                   | -                                    | t-score: -25.9409; p value: 1.80E-145 |
| 1000              | -                                   | t-score: -12.1603; p value: 3.96E-32 | t-score: -16.6006; p value: 3.84E-55  |
| 100               | t-score: -9.0409; p value: 6.75E-15 | t-score: -12.7437; p value: 6.76E-23 | t-score: -14.0958; p value: 1.05E-25  |

To determine whether such a trend also exists in true rather than predicted data, we performed a similar analysis on the observed values in ToxCast. Similar to the analysis for Table S4, we selected the compounds that appeared in both ToxCast and the NCI60 cell lines, calculated their AR antagonist scores using observed values in ToxCast, and did an analysis on top 10 and top 20 compounds. Some of the results are presented in tables S6~S7. While all the breast cancer cell lines in Table S6 have similar results as Table S7, which corresponds to BT-549, only Table S7 is presented as an example.

*Table S6 Mean and standard deviation of logGI50 values in top-n compounds in true AR antagonist scores calculated from observed data in ToxCasts*

| Panel  | top_n | cell line       | mean value | standard deviation |
|--------|-------|-----------------|------------|--------------------|
| Breast | 61    | BT-549          | -4.6962    | 1.0183             |
| Breast | 20    | BT-549          | -5.3118    | 0.8011             |
| Breast | 10    | BT-549          | -5.5317    | 0.9963             |
| Breast | 68    | HS 578T         | -4.7523    | 1.0998             |
| Breast | 20    | HS 578T         | -5.1861    | 0.9444             |
| Breast | 10    | HS 578T         | -5.4974    | 1.1785             |
| Breast | 66    | MCF7            | -4.8324    | 1.1053             |
| Breast | 20    | MCF7            | -5.5127    | 1.0835             |
| Breast | 10    | MCF7            | -5.3829    | 1.0357             |
| Breast | 65    | MDA-MB-231/ATCC | -4.6888    | 0.9834             |
| Breast | 20    | MDA-MB-231/ATCC | -5.2618    | 0.8938             |
| Breast | 10    | MDA-MB-231/ATCC | -5.4224    | 0.9242             |
| Breast | 65    | T-47D           | -4.7342    | 0.9420             |
| Breast | 20    | T-47D           | -5.4541    | 0.8323             |
| Breast | 10    | T-47D           | -5.6247    | 1.0080             |

*Table S7 Base top-k compared against other top-k's for BT-549. A one sample t-test is conducted for each filled entry, where H0 is that both top-k's have identical means, while H1 is that the base top-k has a smaller mean.*

| Cell line: BT-549 | Top-k to compare against           |                                      |
|-------------------|------------------------------------|--------------------------------------|
| Base top-k        | 20                                 | 68                                   |
| 20                | -                                  | t-score: -3.43656; p value: 0.001383 |
| 10                | t-score: -0.698; p value: 0.251406 | t-score: -2.65208; p value: 0.01319  |

Clearly, we can observe that tables S6~S7 are similar to tables S4~S5, top compounds in true AR antagonist scores calculated from observed values also tend to be significantly more active in breast cancer cell lines than lower compounds, similar to their predicted counterparts. This indicates PADME captures the patterns present in the training data.

This kind of trend is similar in other cancer types in NCI60 data, so we can only say that the AR antagonist score we proposed shows the general toxicity of a compound.

### 3.2. Wet-lab experiments on compounds

Nevertheless, we decided to test whether the compounds predicted with high AR antagonist effects are truly so. Because we cannot readily conduct the chemical database search (like in the main text where we were finding the compounds that bind strongly to AR) due to insufficient amount of information available, we decided to purchase the compounds and conduct wet-lab experiments on their AR antagonist performance. We chose 38 compounds from the top predictions that were available from the vendors including the National Cancer Institute, and 3 of them were confirmed to be active after going through eGFP and PSA (Prostate-Specific Antigen) tests. See Table S8 which lists the PSA assay results.

*Table S8 The confirmed active compounds and their PSA assay results (smaller is better). As a reference, MDZ, a state-of-the-art drug, has PSA value of 0.6928.*

| 2D representation                                                                   | ZINC ID     | PSA assay result |
|-------------------------------------------------------------------------------------|-------------|------------------|
| 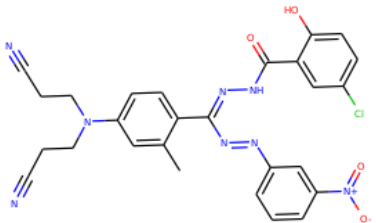 | ZINC8665890 | 2.566            |
| 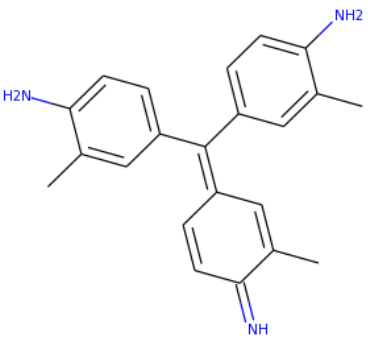 | ZINC3861637 | 4.860            |

|                                                                                   |             |       |
|-----------------------------------------------------------------------------------|-------------|-------|
| 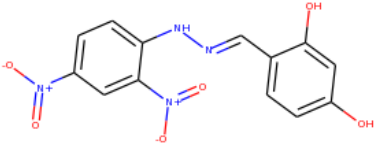 | ZINC4947964 | 6.113 |
|-----------------------------------------------------------------------------------|-------------|-------|

The size of our candidate compound set used for this study is only around 100000, so the choices are limited. 3 actives out of 38 should be a pretty good performance.

### 3.3. Summary

To summarize, we predicted the interaction strength between compounds and androgen receptor (AR), the compounds predicted to have strong antagonist effects with AR indeed showed higher level of activities in NCI60 dataset breast cancer cell lines (and other cancer cell lines), suggesting that PADME has the potential to be applied in drug development. However, contrary to what we believed, the effect of AR seems to be not specific to breast cancer cell lines, but affect all cancer cell lines in general, and our AR antagonist score degenerates to a general toxicity indicator. This could be caused by the extra layer of complexity we introduced when making the formula to calculate AR antagonist score, not necessarily the problem of PADME; instead, PADME faithfully captures the pattern in the training dataset and shows it in the test dataset. Another possible source of problem is that our understanding of AR's effect on cancer cell lines is not complete enough. The review paper by Munoz et al. [25] might provide some justification to our results, since they suggested the influence of AR across a wide variety of cancers which still lack studies.

### References

- 1 Davis, M.I., Hunt, J.P., Herrgard, S., Ciceri, P., Wodicka, L.M., Pallares, G., Hocker, M., Treiber, D.K. and Zarrinkar, P.P., **2011**. Comprehensive analysis of kinase inhibitor selectivity. *Nat. Biotechnol.*, 29(11), p.1046.
- 2 Davis Dataset (Supplementary Tables 3 and 4), <https://www.nature.com/articles/nbt.1990#supplementary-information>. Accessed on June 2, 2017.
- 3 PubChem website, <https://pubchem.ncbi.nlm.nih.gov/>. Accessed on June 2, 2017.
- 4 NCBI Batch Entrez, <https://www.ncbi.nlm.nih.gov/sites/batchentrez>. Accessed on June 3, 2017.
- 5 Metz, J.T., Johnson, E.F., Soni, N.B., Merta, P.J., Kifle, L. and Hajduk, P.J., **2011**. Navigating the kinome. *Nat. Chem. Biol.*, 7(4), p.200.

- 6 *Metz Dataset (Supplementary Table 2)*,  
<<https://www.nature.com/articles/nchembio.530#supplementary-information>>. Accessed on June  
5, 2017.
- 7 *KinBase. The Kinase Database website*, <<http://kinase.com/web/current/kinbase/>>. Accessed on  
June 5, 2017.
- 8 *KinBase. The Kinase Database. Human Kinome Database website*,  
<<http://kinase.com/web/current/kinbase/genes/SpeciesID/9606/>>. Accessed on June 5, 2017.
- 9 Manning, G., Whyte, D.B., Martinez, R., Hunter, T. and Sudarsanam, S., **2002**. The protein  
kinase complement of the human genome. *Science*, 298(5600), pp.1912-1934.
- 10 Tang, J., Sz wajda, A., Shakyawar, S., Xu, T., Hintsanen, P., Wennerberg, K. and Aittokallio, T.,  
**2014**. Making sense of large-scale kinase inhibitor bioactivity data sets: a comparative and  
integrative analysis. *J. Chem. Inf. Model.*, 54(3), pp.735-743.
- 11 *KIBA Dataset (Supplementary File ci400709d\_si\_002.xlsx)*,  
<<https://pubs.acs.org/doi/suppl/10.1021/ci400709d>>. Accessed on June 10, 2017.
- 12 *ChEMBL database (release chembl\_23)*,  
<[http://ftp.ebi.ac.uk/pub/databases/chembl/ChEMBLdb/releases/chembl\\_23/](http://ftp.ebi.ac.uk/pub/databases/chembl/ChEMBLdb/releases/chembl_23/)>. Accessed on June  
10, 2017.
- 13 Gaulton, A., Hersey, A., Nowotka, M., Bento, A.P., Chambers, J., Mendez, D., Mutowo, P.,  
Atkinson, F., Bellis, L.J., Cibrián-Uhalte, E. and Davies, M., **2016**. The ChEMBL database in  
2017. *Nucleic Acids Res.*, 45(D1), pp.D945-D954.
- 14 *ChEMBL webresource client* <[https://github.com/chembl/chembl\\_webresource\\_client](https://github.com/chembl/chembl_webresource_client)>.  
Accessed on June 10, 2017.
- 15 Davies, M., Nowotka, M., Papadatos, G., Dedman, N., Gaulton, A., Atkinson, F., Bellis, L. and  
Overington, J.P., **2015**. ChEMBL web services: streamlining access to drug discovery data and  
utilities. *Nucleic Acids Res.*, 43(W1), pp.W612-W620.
- 16 U.S. EPA. 2018. ToxCast and Tox21 Summary Files invitrodb\_v2. Retrieved from  
<https://www.epa.gov/chemical-research/toxicity-forecaster-toxcasttm-data> on March 22, 2018.  
Data released in October 2015.
- 17 U.S. EPA. 2018. ToxCast & Tox21 Chemicals Distributed Structure-Searchable Toxicity  
Database DSSTox\_20151019. Retrieved from <https://www.epa.gov/chemical-research/toxicity-forecaster-toxcasttm-data>  
on March 22, 2018. Data released in October 2015.
- 18 Molecular Operating Environment (MOE), 2013.08; Chemical Computing Group ULC, 1010  
Sherbooke St. West, Suite #910, Montreal, QC, Canada, H3A 2R7, 2018.
- 19 *UniprotKB website*, <<https://www.uniprot.org/uniprot/>>. Accessed on Mar 25, 2018.
- 20 The UniProt, C. **2016**. UniProt: the universal protein knowledgebase. *Nucleic Acids Res.*, 45,  
D158-D169, doi:10.1093/nar/gkw1099.
- 21 Zhou, Z. (周志华), **2016**. 机器学习(Machine Learning). Qing Hua Da Xue chu ban she  
(Tsinghua University Press).
- 22 Buda, M., Maki, A. and Mazurowski, M.A., **2018**. A systematic study of the class imbalance  
problem in convolutional neural networks. *Neural Networks*, 106, pp.249-259.
- 23 Mina, A., Yoder, R. and Sharma, P., **2017**. Targeting the androgen receptor in triple-negative  
breast cancer: current perspectives. *Oncotargets Ther.*, 10, p.4675.
- 24 Järvelin, K. and Kekäläinen, J., **2002**. Cumulated gain-based evaluation of IR techniques. *ACM  
Transactions on Information Systems (TOIS)*, 20(4), pp.422-446.
- 25 Munoz, J., Wheler, J.J. and Kurzrock, R., **2015**. Androgen receptors beyond prostate cancer: an  
old marker as a new target. *Oncotarget*, 6(2), p.592.
